# Supplementary material for: Politeness Transfer: A Tag and Generate Approach
Source: arXiv:2004.14257 source file (2020-05-01)
Supplement: Supplementary file 1 [file additional_trash.tex]

% \if 0
% In this work, we present a novel text attribute transfer system that performs effective attribute transfer while making minimal changes to the input. Unlike recent style transfer systems, we don't rely on adversarial losses to train our model. Instead, we rely on the key intuition that most attribute transfer tasks require us to perform slight changes to certain parts of the sentences, while retaining most of the information. Further, the changes do not always involve deletion or addition, and may require either and or both the operations. Our system consists of two seq2seq systems, the first one of which is called marker and the other one is called the filler. The marker learns to add markers at locations it thinks need to be changed to perform attribute transfer. These markers may substitute existing words or may serve as a placeholder for adding new words. The filler takes these markers and adds attribute words that finally move the input sentence to the desired attribute. Our system is able to improve on or match the performance on all the existing datasets as given by attribute classifiers, and surpasses all the existing systems on content-preserving metrics by a large margin.

% The goal of our system is to transfer a source sentence into a given style attribute.  While most of the common examples in the literature focus on datasets that go from one attribute to another, another common case where the style transfer has to happen from a source sentence that does not have a specific attribute has received little attention. To this end, we present a new task of politeness transfer the corresponding dataset. Additionally, we evaluate our system on the other widely accepted attribute transfer datasets.

% In order to underscore our model's ability to handle the case of add only changes, we needed a dataset that would have a well defined target attribute class but a fuzzy or ill-defined notion of the other class. While looking for such datasets, not only did we realize that such a dataset does not exist, but we also discovered that the community at large has been focused on attribute transfer for cases wherein both the extremes are well defined. 

% Typical examples include performing attribute transfer on sentiment  (positive vs negative), political narrative (democratic vs republican), gender (male vs female) and the likes. However, these bi-modal cases leave out an important class of attribute transfer that are prevalent in everyday discourse: the cases where the attribute is well defined but it's complement is either not well defined or encompasses everything else (one vs. all). We identify examples of two such kinds of text attributes: racism and politeness. In both the cases, while it is relatively easy to identify and define the examples that have the attribute (racist/polite text), the definition of the complementary set is basically just that: ``not-racist'' and ``not-polite''. Note that we don't focus on cases where the sentence has a curse word and is thus impolite, because they would form non-interesting and trivial examples (and can typically be brought to the neutral zone by a mere deletion of curse words). In order to evaluate our systems on such instances and to bring the attention of the community at large, we curate and release a politeness transfer dataset, derived from the Enron email corpus \cite{klimt2004introducing}.


% To compare our work with the state-of-the-art  approaches  of  style  transfer  for  non-parallel  corpus  we  perform  gender transfer, political slant transfer and sentiment  transfer, replicating the models and experimental setups of \cite{shen2017style}, \cite{prabhumoye-etal-2018-style} and \cite{li-etal-2018-delete}.

% \sm{1. What is politeness, how is it relevant in social interactions, applications \\
% 2. limitations and problems with current methods: content transfer. motivation for our model.\\
% 3. our approach and how we overcome the limitations.\\
% 4. politeness : novel, hard overcome\\
% 5. contributions\\
% 2. applications in which style transfer is used 
% \cite{chandu2019my}, dongyeop story telling dataset.}
% \fi


\if 0
\section{Introduction}
Requests are an important part of everyday human exchange. Further, common courtesy typically demands that the requests be polite. While in-person communication can benefit from non-verbal clues like body language, tone and mannerisms to convey politeness, text exchange has to depend entirely on the choice of words and phrasing to convey a request without sounding too imposing. While a bulk of polite requests are made up of words that explicate the intent of the speaker to be polite by using words like  ``please'' and ``thanks'',  the tail consists of a large number of subtle cues, including but not restricted to words and phrases that intend to indicate the speaker's desire to get the request fulfilled without sounding too imposing on the other party. 

A natural question to ask then is what exactly is a polite request? Clearly, the right answer depends on the culture, language, background and social structure of both the speaker and the addressed person. For practical purposes, we restrict our attention to the notion of politeness as widely accepted between the English speakers in a formal setting in north America. For a linguistically motivated definition, we refer the readers to the (). We focus on a complementary, data-driven definition of politeness as given by (). 

In this work, we set to make progress towards the question ``can we take a request and make it more polite?''. The challenges in tackling such a question are manifold. First, we leverage the data-driven definition of politeness as proposed () to draw a boundary around our definition of politeness. Next, we process a dataset of emails to create a setup that can allow us to show the efficacy of our approach on real world datasets. Like most other style transfer problems, since there is no training data present, and the clues for politeness are subtle and unipolar, we propose a novel system that breaks down the problem of controlled text generation into two parts: a) Our first system, the marker, generates politeness markers that identify locations in the text that can be altered. b) The generators takes cues from the markers and learns to recreate a given sentence to make it more polite. 

Most of the current style transfer techniques tackle the problem of transferring text from one extreme distribution to the other. Prevalent popular examples in the literature include transferring sentiment, gender or political opinion. For each of these examples, the boundaries of each of the classes is relatively well defined. However, in certain cases, like politeness, such extremes are either trivially defined or have a fuzzy boundary. Furthermore, it might not be meaningful to go from the well defined class to the trivial extreme. Consider the example ``send me the data". This sentence is not polite, however, at the same time, it is not impolite. Consider a variant, ``please send me the data", which will be widely accepted to be more polite. We define such class of problems as ``unipolar style transfer".


Our main contributions are as follows:
\begin{itemize}
    \item To the best of our knowledge, no one has presented the problem of poli We release a dataset that contains politeness annotations.
    \item We present politeness as a problem of attribute transfer. 
    \item We highlight the unimodality of politeness; while highlighting something as being polite is easier, the absence of politeness is not necessarily a proof of impolitness. This is in stark contrast with the standard style transfer tasks addressed by the community, in which the distinction is obvious (positive/negative, male/female)
    \item For an email, not every sentence has to be made equally polite. Thus, we need a way to decide the politeness level? [May be something from context?] 
    \item Survey/critic on why regular sentence level style transfers don't work for politeness [and why we choose a delete retrieve based approach.]
    \item Finally we provide a framework which will serve as a baseline for document level politeness transfer.
\end{itemize}

\section{Task Description}
\textbf{4 paragraphs} Talk about what is politeness, talk about what kinds of sentences can be made more polite, why are we focusing on it?, what is the proposed input/output?

\paragraph{Task}
We consider the problem of making a request more polite. For example, given a sentence like ``call me now'', we aim to convert it to a form that would be considered more polite by the addressed person. For this particular case, we aim to transfer the given sentence to something like ``please call me now'' or ``could you please call me now?''.

\paragraph{On uni-polarity of politeness}
Most of the current style transfer techniques tackle the problem of transferring text from one extreme distribution to the other. Prevalent popular examples in the literature include transferring sentiment, gender or political opinion. For each of these examples, the boundaries of each of the classes is relatively well defined. However, in certain cases, like politeness, such extremes are either trivially defined or have a fuzzy boundary. Furthermore, it might not be meaningful to go from the well defined class to the trivial extreme. Consider the example "send me the data". This sentence is not polite, however, at the same time, it is not impolite. Consider a variant, "please send me the data", which will be widely accepted to be more polite. We define such class of problems as ``unipolar style transfer".

\section{A critique of the existing evaluation methods for style transfer}
While it has been long known that automatic metrics are not a very good way of evaluating the performance of NLP systems. During the course of our project, we found that automatic metrics are especially non-informative for politeness transfer. For instance, a system that changes the input sentence by adding a "thank you" in the front would get a very high score on the automatic metrics (BLEU, classifier score). However, from the perspective of achieving the stated goal, such a sentence would be pretty much useless. Thus, just relying on metrics that rely on the surface form or a particular aspect of the system can be extremely misleading. We thus stress that it is very important to not only look at a single automatic metric to evaluate the performance of such systems.

\section{Models}
The masker-unmasker model. Variants:

\begin{itemize}
    \item \textbf{RandomMask $\rightarrow$ Unmask}
    \item \textbf{GMASK $\rightarrow$ Unmask}
    \item \textbf{GMSAK-POS $\rightarrow$ Unmask}
    \item \textbf{GMASK-POS $\rightarrow$ SOFT-BEAM $\rightarrow$ UNMASK}
\end{itemize}
\label{models}


\section{Dataset}

\begin{table}
\centering
\begin{tabular}{llll}
Dataset Name & Style/Attribute                                                                                & Counts - 0 & Counts - 1  \\
Yelp         & \begin{tabular}[c]{@{}l@{}}Sentiment\\\textless{}\textgreater{}(Pos - 1, Neg - 0)\end{tabular} &            &             \\
Amazon       & Sentiment                                                                                      &            &             \\
Enron        & \begin{tabular}[c]{@{}l@{}}Politeness\\\textless{}\textgreater{}(Polite - 1)\end{tabular}      & -          &             \\
             & Gender                                                                                         &            &             \\
             & Political Stance                                                                               &            &             \\
GYAFC        & Formality                                                                                      &            &            
\end{tabular}
\end{table}

\section{Experiments and Results}
\label{sec:length}
evaluation metrics
\input{quantres.tex}

\subsection{Analysis}

% \begin{table}[!htb]
%     \centering
%     \footnotesize
%     \setlength\tabcolsep{4pt}
%     \begin{tabular}{|c|c|c|c|c|c|}\hline
% Model        &       BLEU     &  ROUGE    &   METEOR  &  \thead{Politeness \\ Score} & \thead{Pol \\ Acc} \\ \hline
% DRG-D       &  12.75        &     44.67          &   21.38     &    0.91    &    99.16 \% \\ \hline
% DRG-DR      &   10.63    &     44.96        &   19.96     &      0.8134  &   87.5\% \\ \hline
% \thead{Back \\ Translate}       &        &      &    &     &    \\\hline
% Shen       &        &      &    &    &   \\\hline
% Ours      &     52.53   &    82.7     &  45.35    &   0.6667      &   82.64\%    \\\hline
%     \end{tabular}
%     \caption{\centering{Comparison of our model with popular style transfer methods.}}
%     \label{tab:my_label}
% \end{table}

\section{Related Work}


\section{Conclusion and Future Work}

Some other very important indicators of politeness are casing and punctuation. We don't consider such factors, and focus our attention to the politeness phenomenon induced by words for the following reasons: a) Lack of relevant dataset, b) The lack that such factors play a less important role in the formal communication that we focus on, c) the fact that the effect of casing and punctuation on politeness can be a function the local culture. We leave the exploration of other such clues of politeness for transfer as an important future work.

\bibliography{ref}
\bibliographystyle{acl_natbib}


\newpage

% \nocite{*}

\appendix
\begin{itemize}
    \item We motivate it from a perspective of making email writing easier for people,. Politeness is one aspect which is common when they write an email.
    \item Why different? 1) Nobody has worked on politeness. 
    \item Politeness is a difficult style to transfer. We are working on the domain of emails. Enron data is labelled by a politeness classifier.  
    \item No specific domain.
    \item Unipolar. 
    \item Every sentence can't be made polite.
    \item Knowing when a sentence can me made more polite (and by what degree) is an interesting task by itself.
    \item We don't need delete, retrieve or generate. In fact, our system needs to know when to just add, when to delete, and when to let a sentence flow as is (i.e. without any stylistic transfer).
    \item We are learning the notion of politness from a domain and transferring it to the second domain
\end{itemize}
\fi
